# Supplementary material for: Inverse Bauschinger to Bauschinger Crossover under Steady Shear in Amorphous Solids
Source: arXiv:2512.23313 source file (2025-12-29)
Supplement: Supplementary file 2 [file SM_Healing_SB_PassiveUG.pdf]

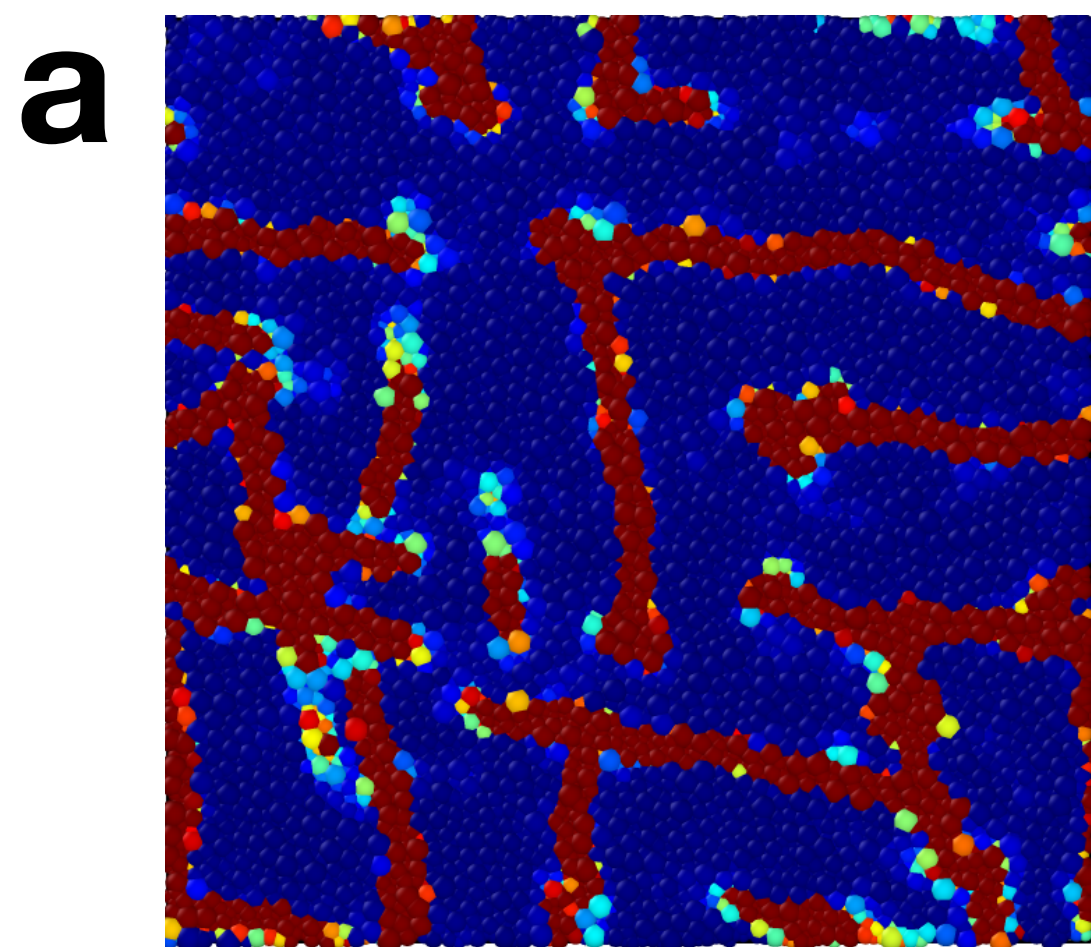

$\sigma = 0.0$

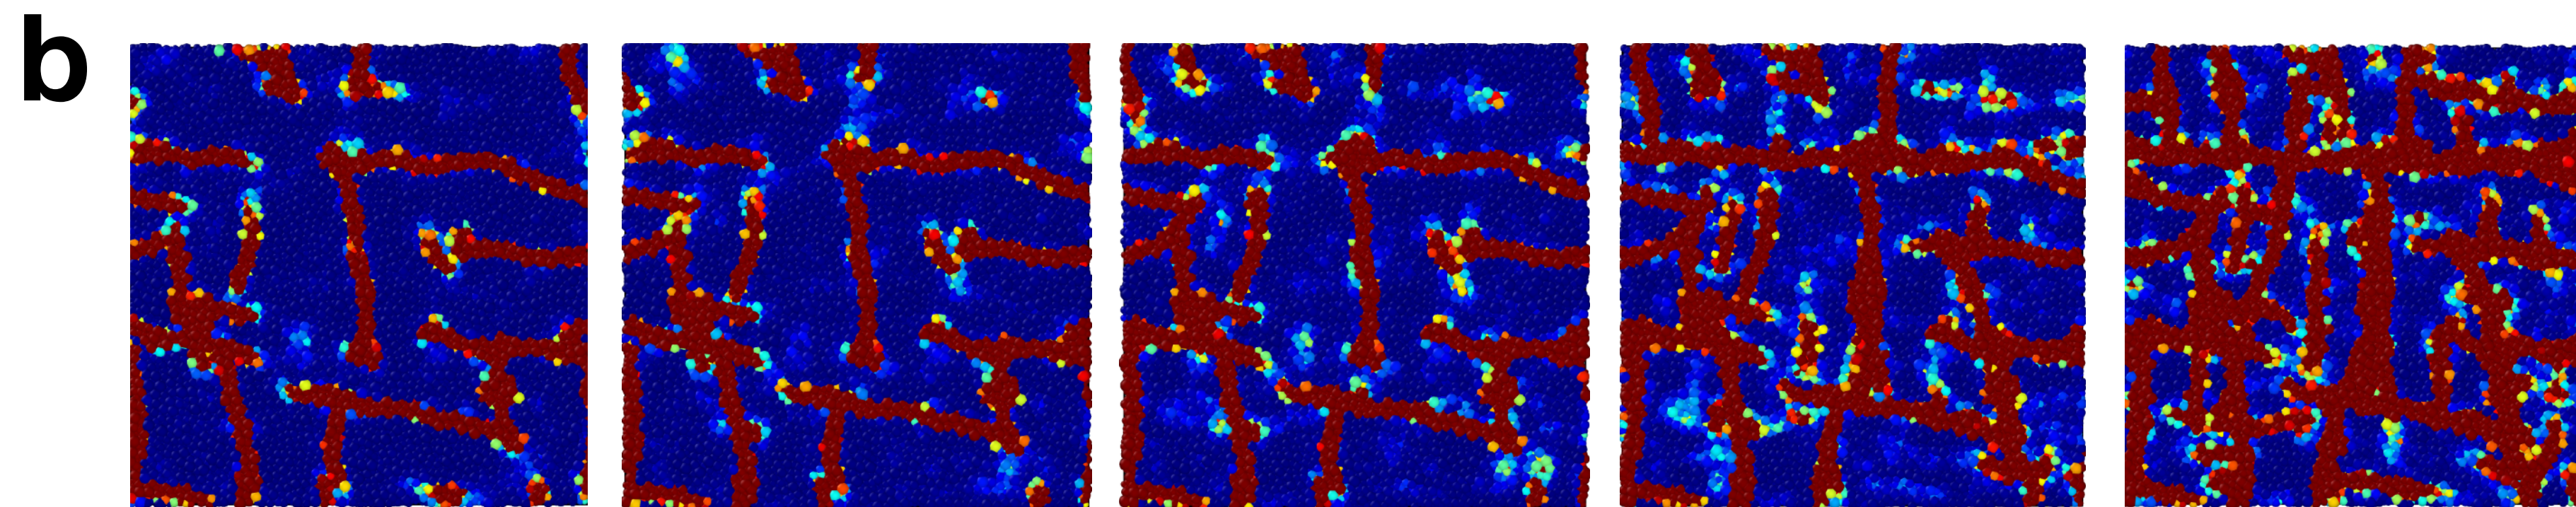

$\gamma = 0.07$

$\gamma = 0.09$

$\gamma = 0.11$

$\gamma = 0.15$

$\gamma = 0.20$

**Positive Shear**

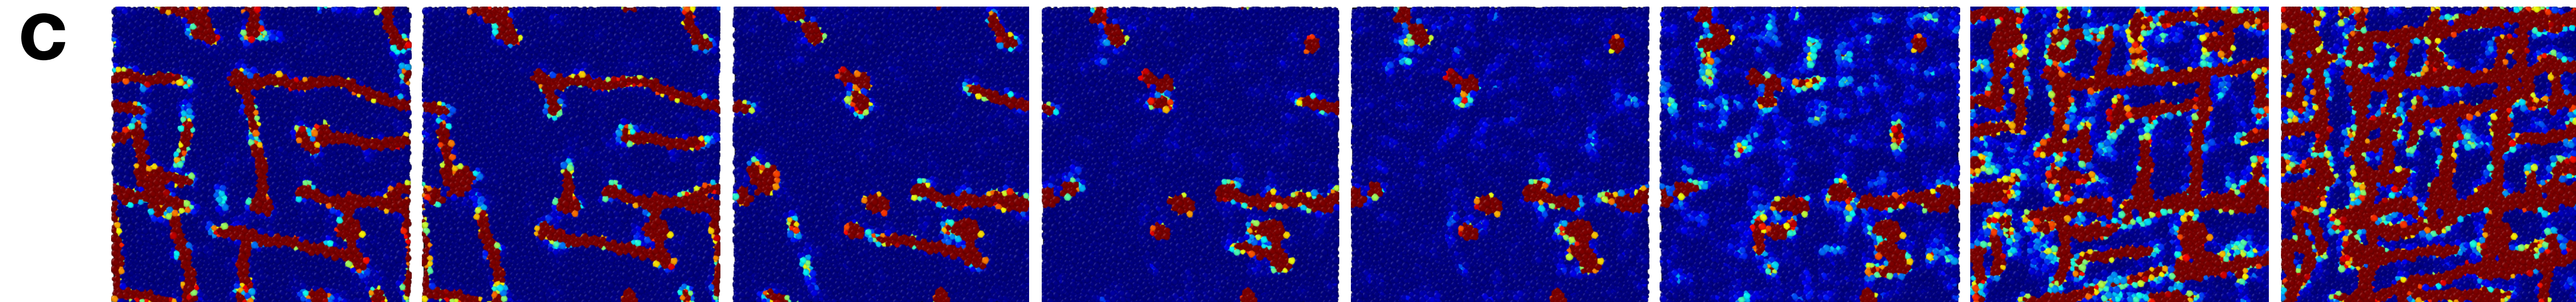

$\gamma = 0.04$

$\gamma = 0.01$

$\gamma = -0.02$

$\gamma = -0.04$

$\gamma = -0.06$

$\gamma = -0.09$

$\gamma = -0.15$

$\gamma = -0.20$

**Negative Shear**

$\gamma_N = 0.15$



**b****Positive  
Shear**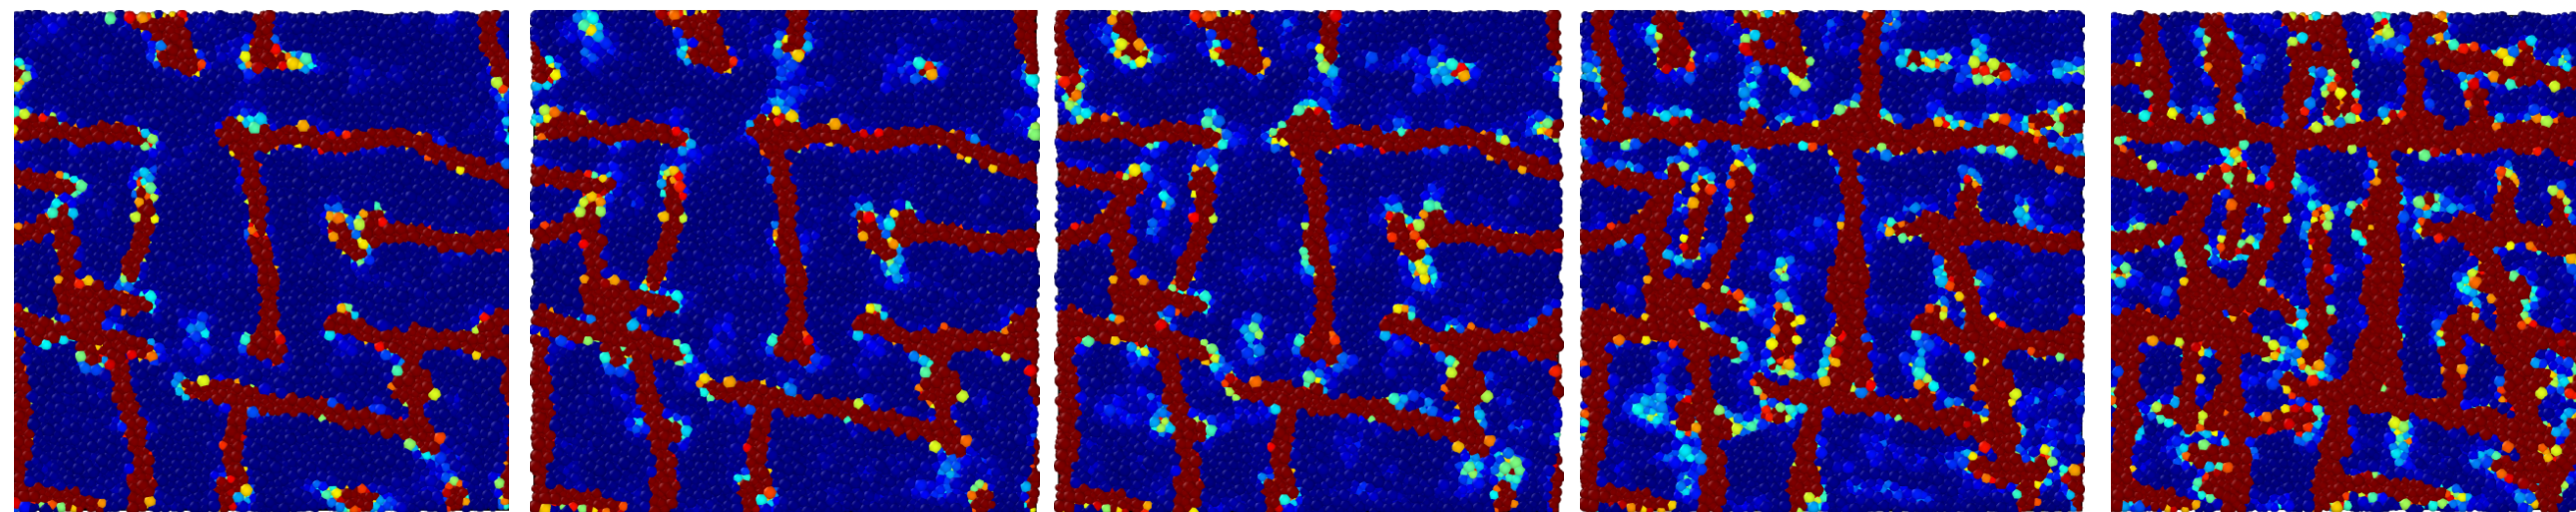

$\gamma = 0.07$

$\gamma = 0.09$

$\gamma = 0.11$

$\gamma = 0.15$

$\gamma = 0.20$

**a**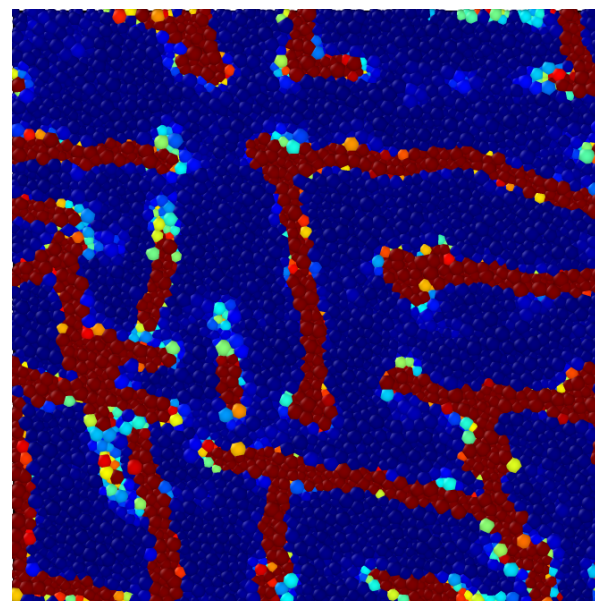

$\sigma = 0.0$

**c**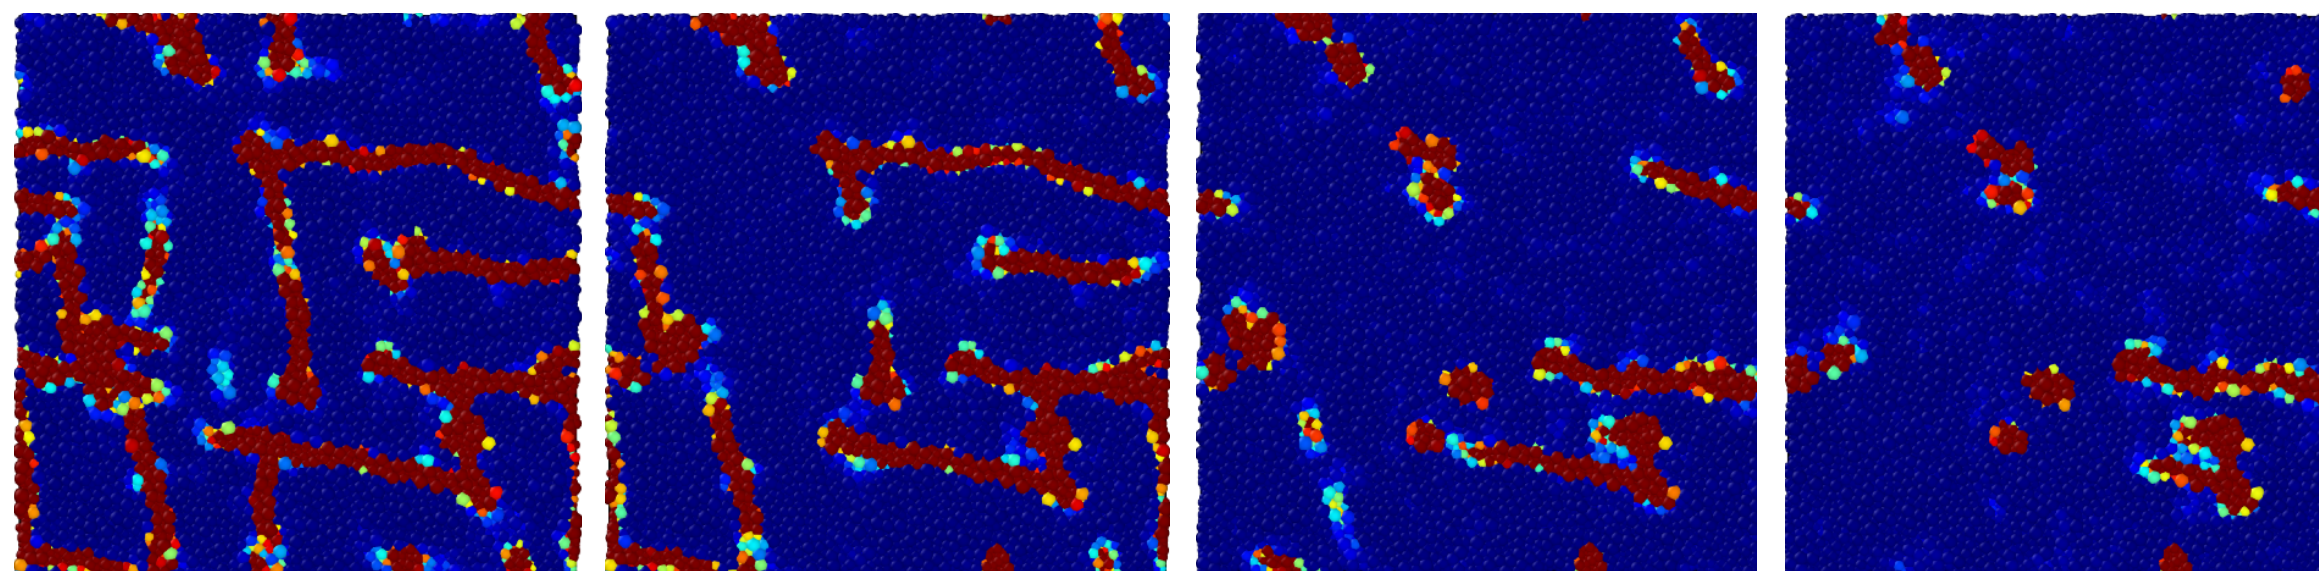

$\gamma = 0.04$

$\gamma = 0.01$

$\gamma = -0.02$

$\gamma = -0.04$

**Negative  
Shear**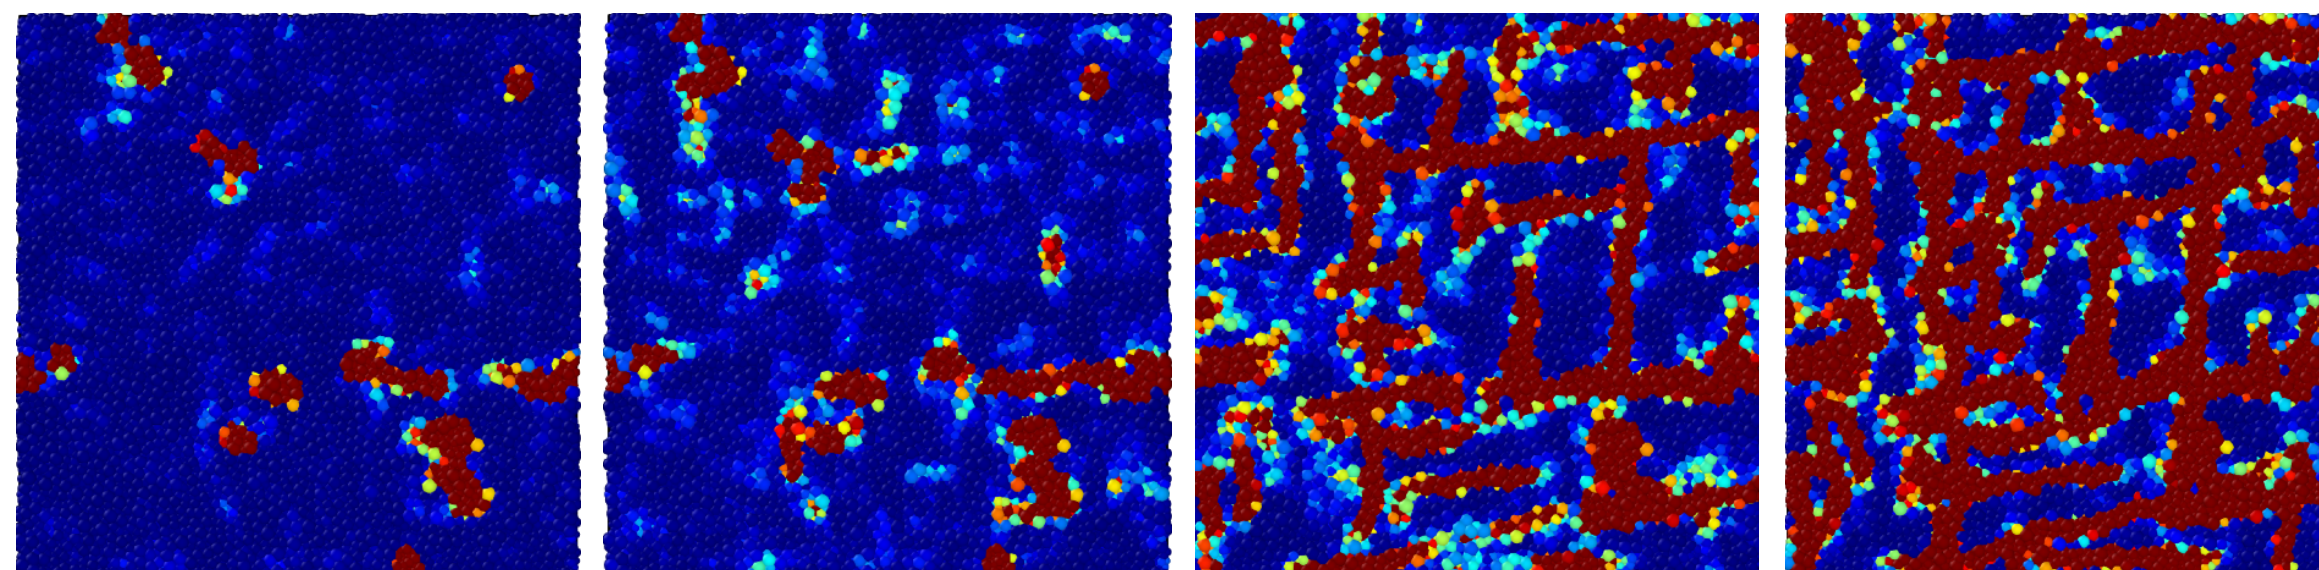

$\gamma = -0.06$

$\gamma = -0.09$

$\gamma = -0.15$

$\gamma = -0.20$

$\gamma_N = 0.15$
